# Supplementary material for: On algorithms to find p-ordering
Source: arXiv:2011.10978 source file (2020-11-22)
Supplement: Supplementary file 1 [file appendix-minimal-repc1.tex]

\section{Proof of Theorem~\ref{thm:uniqueness_of_representation}}
\label{apx:minimal-representation}
%Let there are two representations
Let $rep(S)$ and $\widehat{rep}(S)$ be two representations of a set $S$. 
%Let an element belongs to two different representations in both representations
Let $a\in S$ be an element such that $a\in A_1 \in rep(S)$ and $a\in A_2 \in \widehat{rep}(S)$, such that $A_1=a+p^{k_1}\ast$ and $A_2=a+p^{k_2}\ast$.
%one subset of the other 
Since, $A_1\cap A_2\neq \emptyset$, hence by Observation~\ref{thm:intersect_theorem}, either $A_1 \subset A_2$ or $A_2 \subset A_1$. Without loss of generality, let $A_2 \subset A_1$, that is, $k_1 < k_2$.

%then all elements of bigger set are root
Now since $A_1\in rep(S)$, therefore, $A_1 \subset S$. Hence, the sets $A_2 = a+0\cdot p^{k_2-1}+p^{k_2}\ast$, $A_2+1\cdot p^{k_2-1}=a+1\cdot p^{k_2-1}+p^{k_2}\ast$,..., $A_2+(p-1)\cdot p^{k_2-1}=a+(p-1)\cdot p^{k_2-1}+p^{k_2}\ast$ are all subsets of $S$. Hence, their union, $\bigcup\limits_{b\in [p]} \left(A_2+p^{k_2-1}\cdot b \right)  \subseteq S$. Hence, $\widehat{rep}(S)$ is not minimal.

%hence contradiction
Hence, we've reached a contradiction. Hence, $rep(S)$ is unique.
 \QEDA
